# Supplementary material for: Evidentiality-aware Retrieval for Overcoming Abstractiveness in Open-Domain Question Answering
Source: arXiv:2304.03031 source file (2024-02-01)
Supplement: Supplementary file 1 [file L1_appendix.tex]

\begin{comment}
\begin{wraptable}{r}{7cm}\small
% \begin{table}
 %1.15
\centering
% \begin{wraptable}{r}{0.35\textwidth}
\begin{tabular}{l c c }
 \hline
 \noalign{\hrule height 0.8pt}
    \multirow{2}{*}{\textbf{Retriever}}&\multicolumn{2}{c}{\textbf{NaturalQuestions}}\\
    &top-20 & top-100 \\
\hline
\noalign{\hrule height0.8pt}
     % DPR & 68.39 & 81.25 \\
     DPR & 74.20 & 84.40 \\

\hline
     PiCL &   &   \\
     - $\mathcal{L}_{\texttt{chn}} + \mathcal{L}_{\texttt{cpp}}$ & 74.02 & 84.43 \\ 
     - $\mathcal{L}_{\texttt{chn}} + \mathcal{L}_{\texttt{npr}}$ & 74.27 & 84.57 \\ 
     %PiCL$_{\texttt{L2L3}}$ & - & - \\ 
     - \textbf{$\mathcal{L}_{\texttt{chn}} + \mathcal{L}_{\texttt{cpp}} + \mathcal{L}_{\texttt{npr}}$} & \textbf{76.4} & \textbf{85.18}  \\ 
     
     %PiCL$_{\texttt{L1L2}}$ & 74.02 & 84.43 \\ 
     %PiCL$_{\texttt{L1L3}}$ & 74.27 & 84.57 \\ 
     %PiCL$_{\texttt{L2L3}}$ & - & - \\ 
     %\textbf{PiCL$_{\texttt{L1L2L3}}$} & \textbf{76.4} & \textbf{85.18}  \\ 
     % PiCL$_{\texttt{L1L2L3}}^\dag$ & - & - \\ 
     
     % PiCL$_{\texttt{L1L2}}$ & 67.62 & 80.36 \\ 
     % PiCL$_{\texttt{L1L3}}$ & - & - \\ 
     % PiCL$_{\texttt{L2L3}}$ & - & - \\ 
     
     % PiCL$_{\texttt{L1L2L3}}_{longspan}$ & 69.22 & 81.0 \\ 
     % \textbf{PiCL$_{\texttt{L1L2L3}}$} & \textbf{70.44} & \textbf{81.86}  \\ 
     % PiCL$_{\texttt{L1L2L3}}^\dag$ & 69.31 & 81.39 \\ 
% \hline
%      BM25$^*$ & 59.1 & 73.7  \\ 
%      DPR$_{\texttt{best}}^*$ & 78.4 & 85.4 \\ 
\hline
 \noalign{\hrule height 0.8pt}
 \end{tabular}
 
\caption{Ablation study of ...loss functions... The best result is in \textbf{Bold}. 
% ${^\dag}$ denotes the modified L1 loss, using in-batch counterfactual passages as negatives.  
} 
\label{table:ablationLoss}
% \end{wraptable}
\end{wraptable}
% \end{table}
\end{comment}

\begin{table*}[!ht]\small
% \begin{table}
 %1.15
\centering
% \begin{wraptable}{r}{0.35\textwidth}
\begin{tabular}{l c c c c}
 \hline
 \noalign{\hrule height 0.8pt}
    \multirow{2}{*}{\textbf{Negatives on $(q_i,p_i)$}}&\multicolumn{4}{c}{\textbf{NaturalQuestions}}\\
    &top-1 & top-5 &top-20 & top-100 \\
\hline
\noalign{\hrule height0.8pt}
     % % DPR & 68.39 & 81.25 \\
     % DPR & 74.20 & 84.40 \\

\hline
     $\mathcal{L}_{\texttt{dpr}}$ &   &   \\
     -  $\sum_{j\neq i}p_j$ & 30.44	& 57.84	
     & 75.57	& 85.01\\ 
     -  $\bm{\sum_{j\neq i}p_j + p'_i }$ & \textbf{31.5}	& \textbf{60.03}	& \textbf{76.4}	& \textbf{85.18 }\\ 
     -  $ \sum_{j\neq i}p_j + \sum_{j\neq i}p'_j + p'_i$ & 27.45	& 51.61	& 69.31	& 81.39 \\
      
\hline
 \noalign{\hrule height 0.8pt}
 \end{tabular}
 
\caption{Effect analysis of negative samples on $\mathcal{L}_{\texttt{dpr}}$. The best result is in \textbf{Bold}. $\lambda=0.2$ for $p'$ was used in our setting. 
% ${^\dag}$ denotes the modified L1 loss, using in-batch counterfactual passages as negatives.  
} 
\label{table:L1_appendix}
% \end{wraptable}
\end{table*}
% \end{table}
