# Supplementary material for: Evidentiality-aware Retrieval for Overcoming Abstractiveness in Open-Domain Question Answering
Source: arXiv:2304.03031 source file (2024-02-01)
Supplement: Supplementary file 2 [file appendix_qtype.tex]

\begin{table}[t]\small
 %1.15
\centering

\begin{tabular}{c c | c c}
\hline
\noalign{\hrule height 0.8pt}
     \textbf{Question}& \textbf{Question} & \multicolumn{2}{c}{\textbf{AAR(\%)}} \\
     \cline{3-4}
     \textbf{Type}&\textbf{\#} &DPR&\our~\\
\hline
    Who&547&70.02&80.07\\
    When&295&80.68&87.46\\
    What&228&67.54&77.19\\
    Where&146&65.07&81.51\\
    How&114&71.93&85.09\\
    Which&41&73.17&85.37\\
\hline
\noalign{\hrule height 0.8pt}
\end{tabular}

\caption{AARs of DPR and \our~on various question types. Note that out of 1,382 gold questions, 1,371 were identified by matching interrogative words. }

\label{tab:qtype}
\end{table}
