# Supplementary material for: Evidentiality-aware Retrieval for Overcoming Abstractiveness in Open-Domain Question Answering
Source: arXiv:2304.03031 source file (2024-02-01)
Supplement: Supplementary file 3 [file appendix_qtype_aar.tex]

\begin{table}[t]\small
 %1.15
\centering
\caption{AARs and reader \dahyunadd{Exact Match scores }of DPR and DPR+PiCL on various question types. Note that \dahyunadd{3,429 out of 3,610 questions and 1,371 out of 1,382 gold questions are used for reader inference and AARs, } 
% 1,382 gold questions, 1,371 were 
identified by matching interrogative words. \dahyunadd{Top-5 retrieved passages are used for DPR reader inference.}}
\begin{tabular}{c |c | c c c c}
\hline
\noalign{\hrule height 0.8pt}
     \textbf{Question}& {\textbf{\# Questions}} & \multicolumn{2}{c}{\textbf{AAR(\%)}} & \multicolumn{2}{c}{\textbf{Exact Match (EM)}}\\
     \cline{3-4} \cline{5-6}
     \textbf{Type}&\textbf{(Gold)}&DPR&DPR+PiCL&DPR&DPR+PiCL \\
\hline
    How&246 (114)&71.93&{85.09}&32.52&{34.15}\\
    What&585 (228)&67.54&{77.19}&22.91&{24.27}\\
    When&710 (295)&80.68&{87.46}&33.66&{36.34}\\
    Where&408 (146)&65.07&{81.51}&28.68&{32.84}\\
    Which&125 (41)&73.17&{85.37}&24.00&{25.60}\\
    Who&1355 (547)&70.02&{80.07}&40.66&{43.03}\\
\hline
\noalign{\hrule height 0.8pt}
\end{tabular}

\label{tab:qtype}
\end{table}
