# Supplementary material for: Evidentiality-aware Retrieval for Overcoming Abstractiveness in Open-Domain Question Answering
Source: arXiv:2304.03031 source file (2024-02-01)
Supplement: Supplementary file 4 [file appendix_qtype_em.tex]

\begin{table*}[t]\small
 %1.15
\centering
\begin{tabular}{c  c | c c |c c}
\hline
\noalign{\hrule height 0.8pt}
     \textbf{Question}& {\textbf{Question}} & \multicolumn{2}{c|}{\textbf{Top-5 Accuracy}} & \multicolumn{2}{c}{\textbf{Exact Match (EM)}}\\
     \cline{3-4} \cline{5-6} 
     \textbf{Type}&\textbf{\#} &DPR&\our~&DPR&\our~\\
\hline
    Who&1355 &63.99&72.84 &40.66&{43.03} (+2.37) \\
    When&710 &57.32&68.59 &33.66&{36.34} (+2.68) \\
    What&585 &53.85&60.68 &22.91&{24.27} (+1.36) \\
    Where&408 &58.09&75.74 &28.68&{32.84} (+4.16)\\
    How&246 &57.32&65.85 &32.52&{34.15} (+1.63) \\
    Which&125 &68.00&68.80 &24.00&{25.60} (+1.60) \\
    
\hline
\noalign{\hrule height 0.8pt}
\end{tabular}
\caption{{End-to-end QA performance (EM) and retriever top-5 accuracy} on various question types. Note that
% {3,429 out of 3,610 questions are used, and} 
% identified by matching interrogative words. 
{we switch retrieved passages from DPR or \our~on same DPR reader for inference.}}

\label{tab:qtype-em}
\end{table*}
